# Supplementary material for: CoReQA: Uncovering Potentials of Language Models in Code Repository Question Answering
Source: arXiv:2501.03447 source file (2025-01-07)
Supplement: Supplementary file 1 [file appendix.tex]

\appendix

\subsection{Prompts used in RepoQA-\small{Bench}}

\subsubsection{Prompt for issue intent classification}

\begin{figure}[ht]
    \centering
    \includegraphics[width=0.95\linewidth]{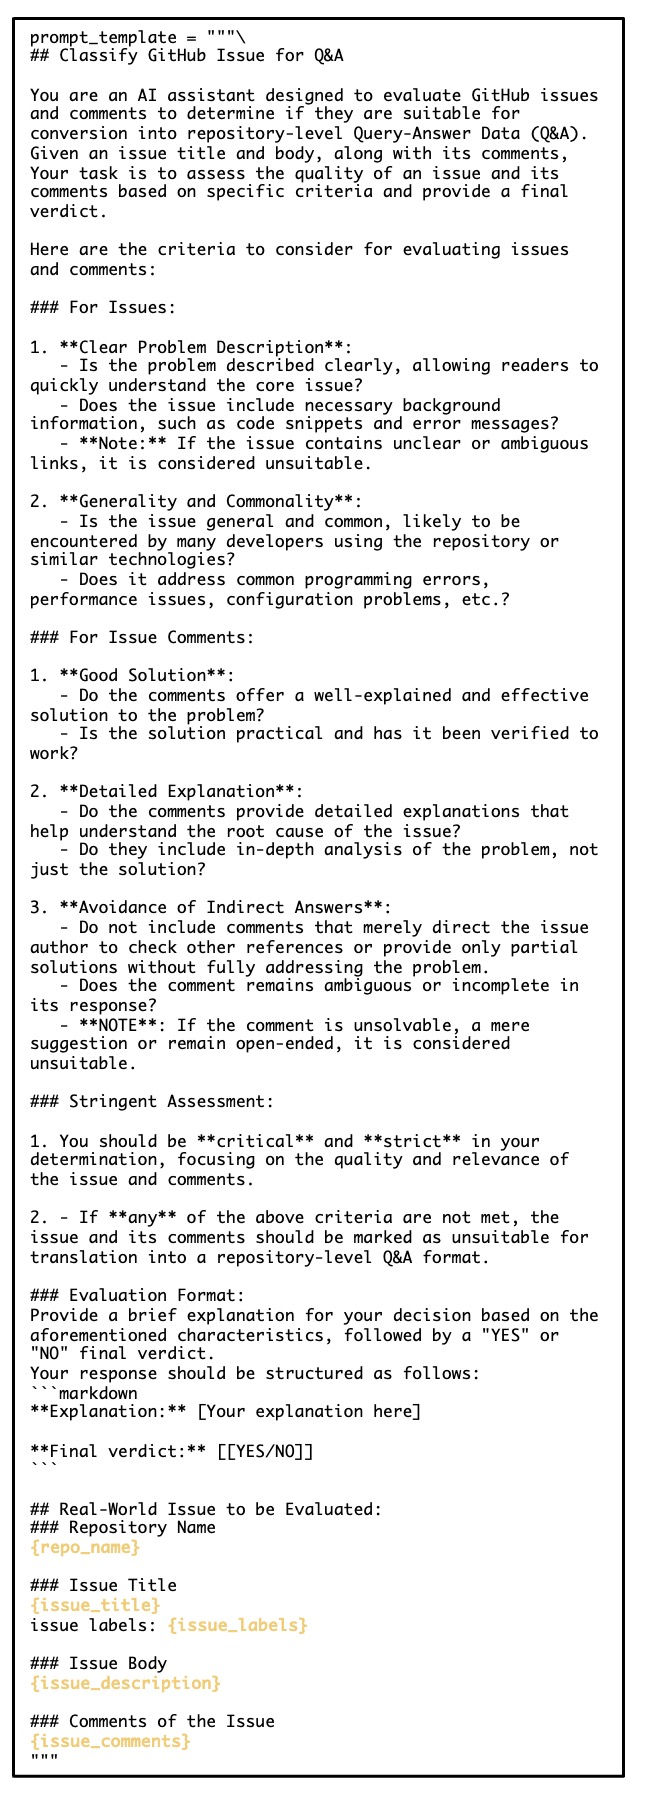}
    \caption{Issue filtering prompt}
    \label{fig:issue_intent_classification_prompt}
\end{figure}

Fig.~\ref{fig:issue_intent_classification_prompt} presents the prompt used for issue intent classification.
In this prompt, we clarify the intent categories and highlight the required output format. 
Additionally, we provide rules for the LLM to analyze the provided content using the chain-of-thought prompt strategy.
The strings surrounded by curly braces in yellow indicate content that will be replaced with specific information from the collected information. 
These placeholders include the repository name (``repo\_name"), the primary programming language used in the repository (``repo\_language"), the issue title (``issue\_title"), the issue labels (``issue\_labels"), and the issue description (``issue\_description").

\subsubsection{Prompt for issue rewrite}

\begin{figure} [th!]
    \centering
    \includegraphics[width=0.95\linewidth]{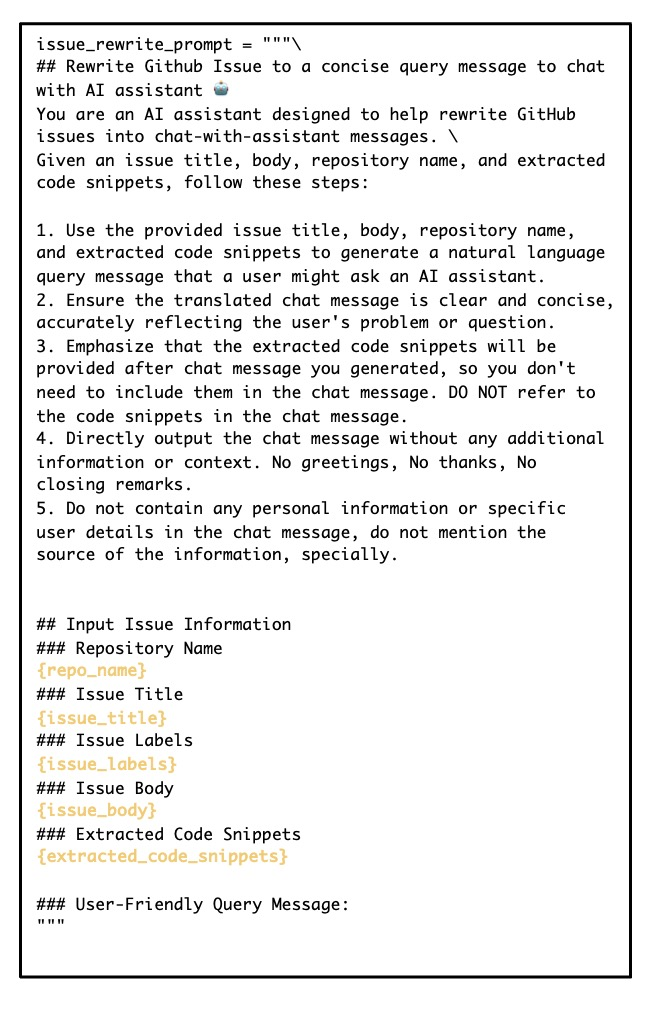}
    \caption{Issue rewrite prompt}
    \label{fig:issue_rewrite_prompt}
\end{figure}

Fig.~\ref{fig:issue_rewrite_prompt} gives our prompt for rewrite the issues into questions.
As is introduced in \S\ref{sec:construction}, we will use repository name (``repo\_name"), issue title (``issue\_title") and issue description (``issue\_description") to generate questions.

\subsubsection{Prompt for reference answer generation}

% \begin{figure}[t!]
%     \centering
%     \includegraphics[width=0.95\linewidth]{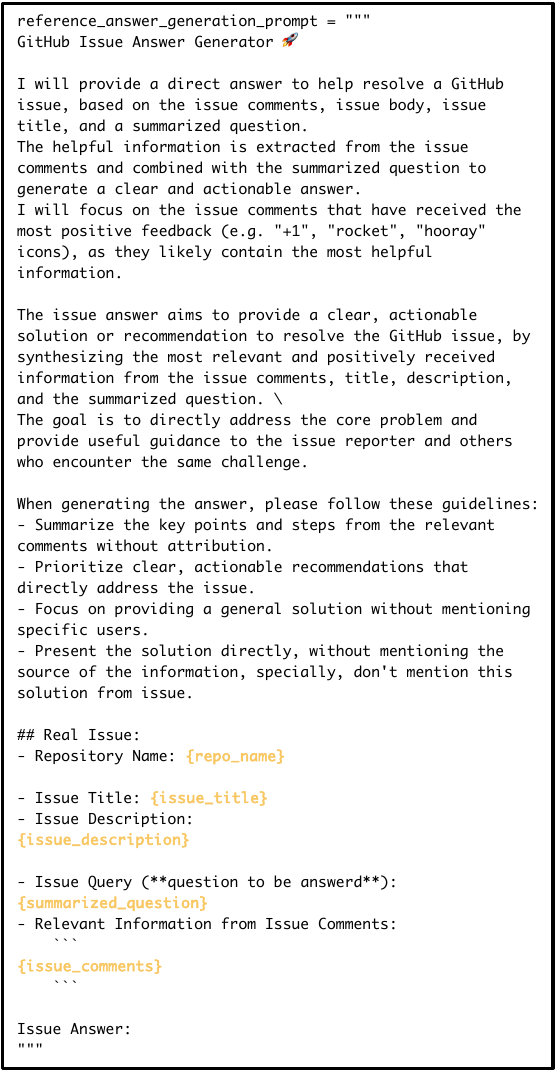}
%     \caption{Reference answer generation prompt}
%     \label{fig:ref-ans-gen-prompt}
% \end{figure}

Fig.~\ref{fig:ref-ans-gen-prompt} illustrates the prompt for generating reference answers combing repository name (``repo\_name"), issue title (``issue\_title"), generated questions (``summarized\_question") and issue comments (``issue\_comments").

\subsubsection{Prompt for absolute quality evaluation}

\begin{figure}[t!]
    \centering
    \includegraphics[width=1\linewidth]{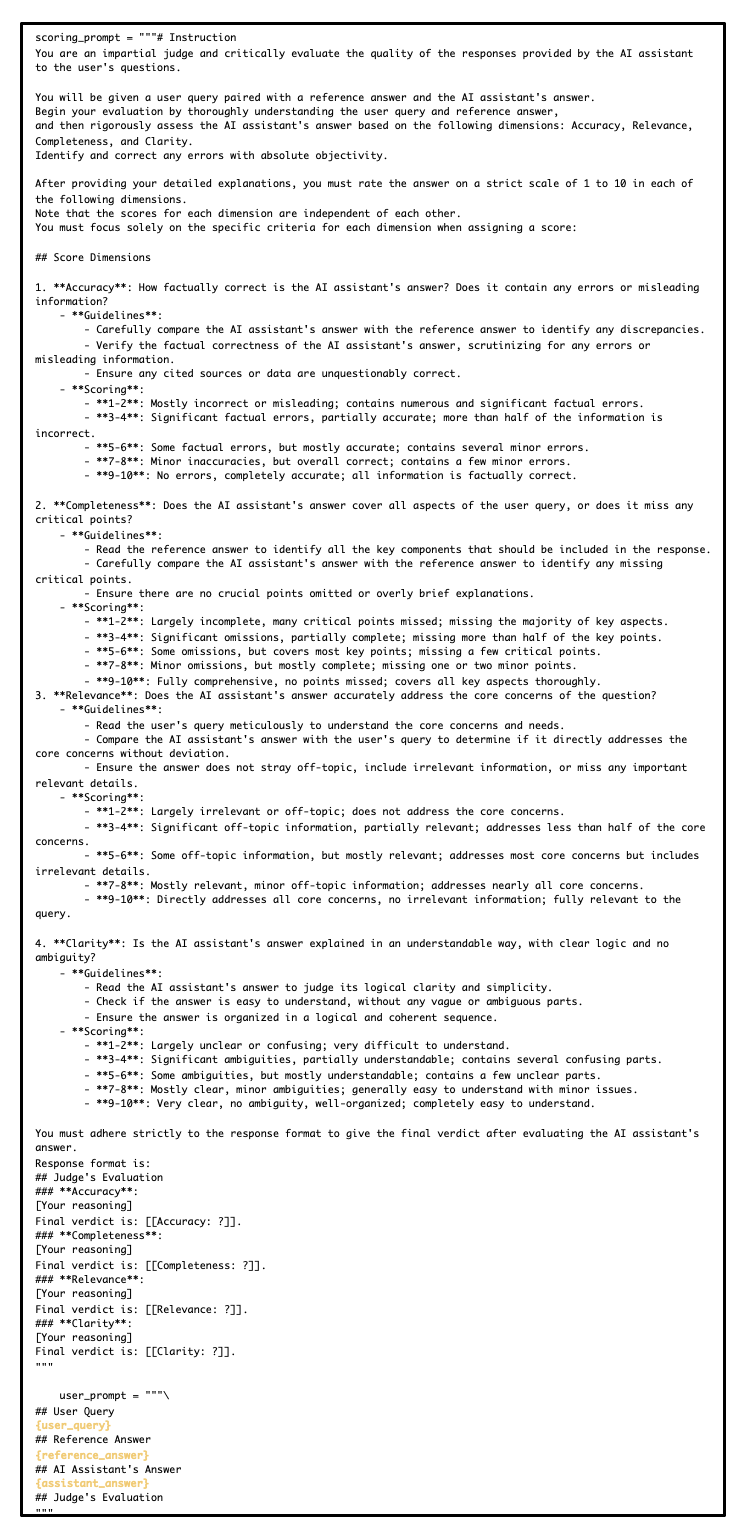}
    \caption{Absolute quality evaluation prompt}
    \label{fig:abs-quality-prompt}
\end{figure}

Fig.~\ref{fig:abs-quality-prompt} gives the prompt for llm-as-a-judge with absolute qulity evaluation. 
We instruct the LLM to understand the question and reference answer, analyze the generated answer, and provide reasons for assigning a particular score. 
The prompt takes the question, reference answers, and generated answers as input, and outputs three metrics along with the corresponding scoring reasons.

\subsubsection{Prompt for pairwise comparison evaluation}

\begin{figure}[t!]
    \centering
    \includegraphics[width=1\linewidth]{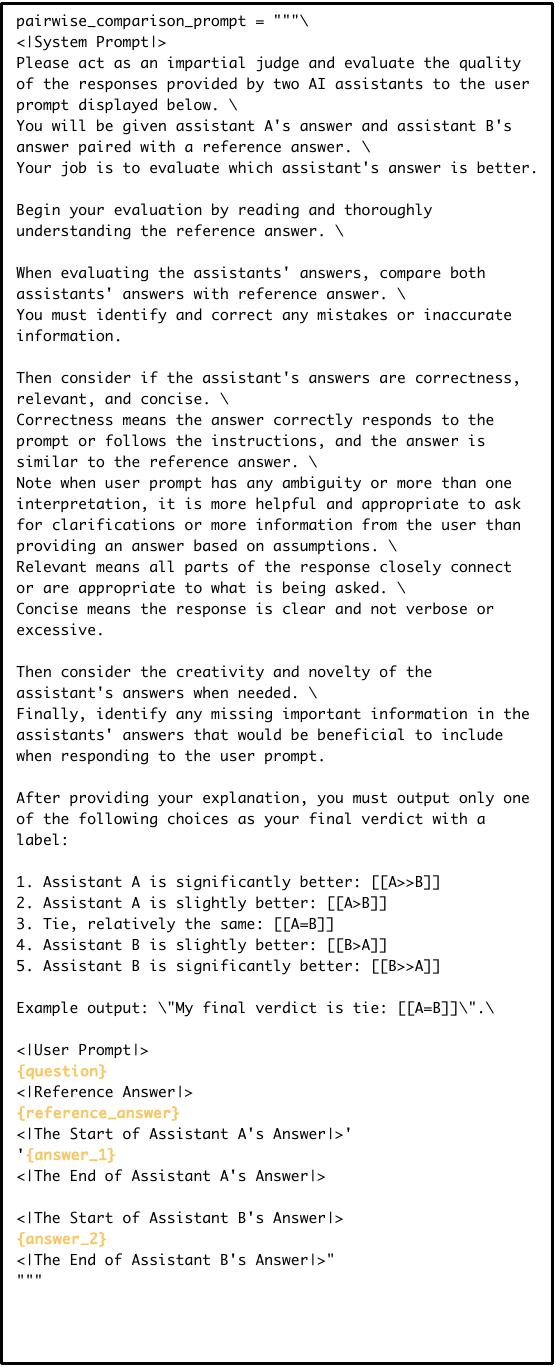}
    \caption{Pairwise comparison evaluation prompt}
    \label{fig:pairwise-judge-prompt}
\end{figure}

Fig.~\ref{fig:pairwise-judge-prompt} gives the prompt for pairwise comparison evaluation.
We integrate the question, reference answer, and two comparison answers into the prompt. 
We use the prompt to instruct the LLM to understand the question and corresponding answers in order to evaluate the two answers being compared.
